# Supplementary material for: Rank Position Forecasting in Car Racing
Source: arXiv:2010.01707 source file (2020-10-23)
Supplement: Supplementary file 1 [file appendix.tex]

\begin{table}
\centering
\caption{Shortterm rank position forecasting}
\label{tbl:rank_forecasting}
\arrayrulecolor[rgb]{0.8,0.8,0.8}
\begin{tabular}{l l l l l l l l l} 
\hline
Dataset      & Model          & Top1Acc & MAE  & rmse & r2   & 10-risk & 50-risk & 90-risk  \\ 
\hline
Indy500-2018 & CurRank        & 0.72    & 1.34 & 3.25 & 0.85 & 0.097   & 0.097   & 0.097    \\ 
\hline
             & DeepAR         & 0.66    & 2.07 & 3.82 & 0.80 & 0.092   & 0.156   & 0.096    \\ 
\hline
             & RankNet-oracle & 0.85    & 0.88 & 2.09 & 0.94 & 0.044   & 0.066   & 0.037    \\ 
\hline
             & RankNet-MLP    & 0.77    & 1.24 & 2.95 & 0.88 & 0.053   & 0.086   & 0.057    \\ 
\hline
             &                &         &      &      &      &         &         &          \\ 
\hline
Indy500-2019 & CurRank        & 0.73    & 1.16 & 3.05 & 0.88 & 0.080   & 0.080   & 0.080    \\ 
\hline
             & DeepAR         & 0.59    & 1.71 & 3.48 & 0.84 & 0.069   & 0.121   & 0.075    \\ 
\hline
             & RankNet-oracle & 0.82    & 0.81 & 1.98 & 0.95 & 0.035   & 0.059   & 0.031    \\ 
\hline
             & RankNet-MLP    & 0.80    & 1.10 & 2.82 & 0.90 & 0.045   & 0.073   & 0.046    \\
\hline
\end{tabular}
\arrayrulecolor{black}
\end{table}

\begin{table}
\centering
\caption{Change of rank position between pitstops}
\arrayrulecolor[rgb]{0.8,0.8,0.8}
\begin{tabular}{|r|r|r|r|r|} 
\hline
Dataset                & Model          & SignAcc                            & MAE                                & rmse                                \\ 
\hline
Indy500-2018           & CurRank        & 0.11                               & 4.04                               & 5.46                                \\ 
\hline
\multicolumn{1}{|l|}{} & RandomForest   & 0.68                               & 3.70                               & 4.98                                \\ 
\hline
\multicolumn{1}{|l|}{} & SVM            & 0.69                               & 3.90                               & 5.28                                \\ 
\hline
\multicolumn{1}{|l|}{} & XGBoost        & 0.54                               & 3.67                               & 5.00                                \\ 
\hline
\multicolumn{1}{|l|}{} & RankNet-oracle & 0.71                               & 3.15                               & 4.83                                \\ 
\hline
\multicolumn{1}{|l|}{} & RankNet-MLP    & {\cellcolor[rgb]{0.8,0.8,0.8}}0.62 & {\cellcolor[rgb]{0.8,0.8,0.8}}3.71 & {\cellcolor[rgb]{0.8,0.8,0.8}}5.41  \\ 
\hline
Indy500-2019           & CurRank        & 0.16                               & 4.27                               & 6.45                                \\ 
\hline
                       & RandomForest   & 0.59                               & 4.40                               & 5.93                                \\ 
\hline
                       & SVM            & 0.59                               & 4.14                               & 6.26                                \\ 
\hline
                       & XGBoost        & 0.56                               & 4.79                               & 6.53                                \\ 
\hline
                       & RankNet-oracle & 0.63                               & 3.58                               & 5.71                                \\ 
\hline
                       & RankNet-MLP    & {\cellcolor[rgb]{0.8,0.8,0.8}}0.49 & {\cellcolor[rgb]{0.8,0.8,0.8}}4.42 & {\cellcolor[rgb]{0.8,0.8,0.8}}6.37  \\
\hline
\end{tabular}
\arrayrulecolor{black}
\end{table}

\iffalse
\begin{wrapfigure}{l}{0.5\textwidth}
  \begin{center}
    \includegraphics[width=\linewidth]{fig/deepar_arch_train.png}
  \end{center}
    \caption{Probabilistic forecasting with autoregressive recurrent network.\cite{salinas_deepar_2019}}
    \label{fig:deepar_arch_train}
\end{wrapfigure}
\fi

\begin{table}
\centering
\caption{Short-term rank position forecasting(prediction leghth=2, dataset=Indy500-2018)}
\label{tbl:rank_forecasting}
\begin{tabular}{l l l l l l l l} 
\hline
Model          & Top1Acc & MAE  & RMSE & R2   & 10-risk & 50-risk & 90-risk  \\ 
\hline
CurRank        & 0.72    & 1.34 & 3.25 & 0.85 & 0.097   & 0.097   & 0.097    \\ 
DeepAR         & 0.66    & 2.07 & 3.82 & 0.80 & 0.092   & 0.156   & 0.096    \\ 
RankNet-Oracle & \textbf{0.85}    & \textbf{0.88} & \textbf{2.09} & \textbf{0.94} & \textbf{0.044}   & \textbf{0.066}   & \textbf{0.037}  \\ 
RankNet-MLP    & 0.77    & 1.24 & 2.95 & 0.88 & 0.053   & 0.086   & 0.057    \\ 
\hline
\end{tabular}
\end{table}

\begin{wraptable}{l}{0.5\textwidth}
\tiny
%\begin{table}
\centering
\caption{Change of rank position between pitstops}
\label{tbl:rank_change}
\begin{tabular}{ l l l l} 
\hline
Model          & SignAcc    & MAE     & RMSE        \\ 
\hline
CurRank        & 0.11       & 4.04    & 5.46     \\ 
RandomForest   & 0.68      & 3.70     & 4.98     \\ 
SVM            & 0.69     & 3.90     & 5.28                                \\ 
XGBoost        & 0.54     & 3.67     & 5.00                                \\ 
RankNet-Oracle & 0.71     & 3.15     & 4.83                                \\ 
RankNet-MLP    & 0.62 & 3.71 & 5.41  \\ 
\hline
\end{tabular}
%\end{table}
\end{wraptable}

\section{Models}

\subsection{Encoder-decoder framework and probabilistic forecasting}

\begin{figure*}[ht]
\centering
\includegraphics[width=0.95\linewidth]{fig/RankNet_all_v2}
\caption{RankNet architecture (a)Cause effects decomposition. History data first feed into PitModel to get RaceStatus in the future, then feed into RankModel to get Rank forecasting. The output of the models are samples drawed from the learned distribution. (b)PitModel is a MLP predicting next pit stop lap given features of current pitage and cautionlaps. (c)RankModel is  2-layers LSTM encoder-decoder predicting rank for next prediction\_len laps, given features of Rank and RaceStatus history, carid and lapstatus predicted by PitModel. }
\label{fig:arch}
\end{figure*}

%Furthermore, due to the capability of probabilistic forecasting, the output of target variable are realizations of a distribution.  

\begin{wraptable}{l}{0.55\textwidth}
\small
%\begin{table}
\centering
\caption{Change of rank position between pitstops}
\label{tbl:rank_change}
\begin{tabular}{c|cc|cc} 
\hline
Dataset        & \multicolumn{2}{c|}{Indy500-2018} & \multicolumn{2}{c}{Indy500-2019}  \\ 
\hline
Model          & SignAcc & MAE                     & SignAcc & MAE                      \\ 
\hline
CurRank        & 0.11    & 4.04                    & 0.16    & 4.27                     \\ 
RandomForest   & 0.68    & 3.70                    & 0.59    & 4.40                     \\ 
SVM            & 0.69    & 3.90                    & 0.59    & 4.14                     \\ 
XGBoost        & 0.54    & 3.67                    & 0.56    & 4.79                     \\ 
RankNet-oracle & 0.71    & 3.15                    & 0.63    & 3.58                     \\ 
RankNet-MLP    & 0.62    & 3.71                    & 0.49    & 4.42                     \\
\hline
\end{tabular}
%\end{table}
\end{wraptable}

\begin{table}
\small
\centering
\caption{Short-term rank position forecasting(prediction leghth=2)}
\label{tbl:rank_forecasting}
\begin{tabular}{l|llll|llll} 
\hline
Dataset   & \multicolumn{4}{c|}{Indy500-2018} & \multicolumn{4}{c}{Indy500-2019}  \\ 
\hline
Model          & Top1Acc & MAE  & 50-Risk & 90-Risk        & Top1Acc & MAE  & 50-Risk & 90-Risk         \\ 
\hline
CurRank        & 0.72    & 1.34 & 0.097   & 0.097          & 0.73    & 1.16 & 0.080   & 0.080           \\ 
DeepAR         & 0.66    & 2.07 & 0.156   & 0.096          & 0.59    & 1.71 & 0.121   & 0.075           \\ 
RandomForest	& 0.51	& 1.75	& 0.000	& 0.000& 	0.62& 	1.33	& 0.000	& 0.000\\
SVM	& 0.72	& 1.34	& 0.000	& 0.000	& 0.73	& 1.18	& 0.000	& 0.000 \\
XGBoost	& 0.46	& 1.63	& 0.000	& 0.000	& 0.64	& 1.25	& 0.000	& 0.000 \\
RankNet-Joint	&0.73	&1.75	&0.14	&0.09	&0.68	&1.63	&0.116	&0.073 \\
RankNet-Oracle & 0.85    & 0.88 & 0.066   & 0.037          & 0.82    & 0.81 & 0.059   & 0.031           \\ 
RankNet-MLP    & 0.77    & 1.24 & 0.086   & 0.057          & 0.80    & 1.10 & 0.073   & 0.046           \\
\hline
\end{tabular}
\arrayrulecolor{black}
\end{table}

\begin{wraptable}{l}{0.55\textwidth}
\small
%\begin{table}
\centering
\caption{Change of rank position between pitstops}
\label{tbl:rank_change}
\begin{tabular}{c|cc|cc} 

\hline
Dataset        & \multicolumn{2}{c|}{Indy500-2018} & \multicolumn{2}{c}{Indy500-2019}  \\ 
\hline
Model          & SignAcc & MAE                     & SignAcc & MAE                      \\ 
\hline
CurRank        & 0.10    & 4.32                    & 0.16    & 4.22                     \\ 
RandomForest   & 0.62    & 3.41                    & 0.57    & 4.00                     \\ 
SVM            & 0.62    & 3.48                    & 0.58    & 4.74                     \\ 
XGBoost        & 0.59    & 3.63                    & 0.57    & 4.38                     \\ 
RankNet-oracle & 0.71    & 3.15                    & 0.63    & 3.58                     \\ 
RankNet-MLP    & 0.66    & 3.73                    & 0.51    & 3.86                     \\
\hline
\end{tabular}
%\end{table}
\end{wraptable}

\subsection{Variable length of rank position forecasting}
\iffalse
\begin{wrapfigure}{l}{0.5\textwidth}
  \begin{center}
    \includegraphics[width=\linewidth]{fig/ranknet-forecasting}
  \end{center}
    \caption{Forecasting rank positions between two pit stops. }
    \label{fig:simulation}
\end{wrapfigure}
\fi

A rank position forecasting network is trained with a fixed prediction length. 
In order to deliver a variable length prediction, e.g., in predicting the rank positions between two pit stops, we apply a fixed length forecasting regressively by using previous output as input for the next prediction. 

%Fig. \ref{fig:arch}(c) illustrates this process by an example race with three cars, where \emph{prediction length} equals two laps. 
At current lap $t$, the historical data for each car are feed into RankNet, future LapStatus are predicted by the pitstop model, and the rank position of the next two laps can be obtained by sorting the target variables of all the cars $Z_{i,t+1:t+2}$. 
%LapStatus is modeled by the pitstop model, either the encoder-decoder network or the separate MLP network. 
Moving current lap forward, RankNet continues forecasting for the next two laps until reaching the farthest next pit stop.

\begin{figure*}[ht]
\centering
\includegraphics[width=0.35\linewidth]{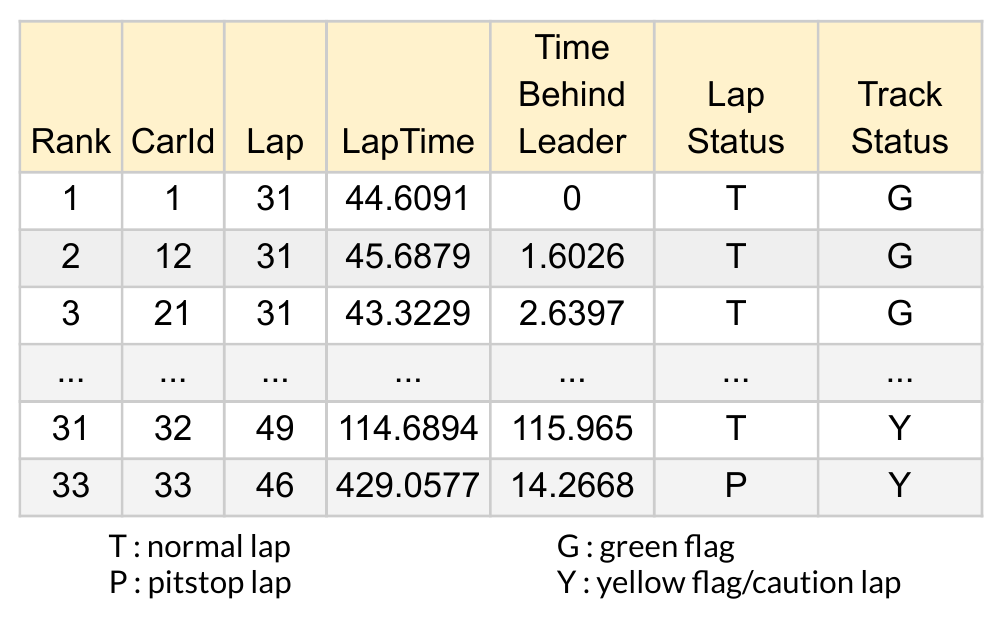}
\includegraphics[width=0.5\linewidth]{fig/laptime_rank_pitstop.pdf}
\caption{Data examples of Indy500-2018. (a)Rank can be calculated by LapTime and TimeBehindLeader. LapStatus and TrackStatus indicate racing status of pitstops and cuation laps. (b) Rank and LapTime sequence of car12, the final winner. Sequence dynamics correlate to racing status.}
\label{fig:indycar_data}
\end{figure*}

\begin{table}
	\caption{MLP PitModel performance comparison}
	\label{tab:pitmodel-cmp}
	\centering
	\begin{tabular}{l|l|rrrr} 
		\hline
		Uncertainty & TrainSet               & \multicolumn{1}{l}{MAE} & \multicolumn{1}{l}{F1@2laps} & \multicolumn{1}{l}{50-Risk} & \multicolumn{1}{l}{90-Risk}  \\ 
		\hline
		with        & select & 4.90                     & 0.63                          & 0.262                        & 0.243                          \\
		with        & all                    & 6.57                     & 0.63                          & 0.353                        & 0.076                          \\
		w/o         & select & 4.90                     & 0.55                          & 0.262                        & 0.445                          \\
		w/o         & all                    & 121.62                   & 0.49                          & 6.524                        & 1.305                         \\
		\hline
		
	\end{tabular}
\end{table}

\iffalse

%\begin{table*}[ht]
%\small
%\centering
%\caption{Short-term rank position forecasting(prediction leghth=2)}
%\label{tbl:rank_forecasting}
%\begin{tabular}{l|llll|llll} 
%\hline
%Dataset   & \multicolumn{4}{c|}{Indy500-2018} & \multicolumn{4}{c}{Indy500-2019}  \\ 
%\hline
%Model          & Top1Acc & MAE  & 50-Risk & 90-Risk        & Top1Acc & MAE  & 50-Risk & 90-Risk         \\ 
%\hline
%CurRank        & 0.72    & 1.34 & 0.097   & 0.097   & 0.73    & 1.16 & 0.080   & 0.080    \\ 
%ARIMA	& 0.68	& 2.63	& 0.097	& 0.087	& 0.57	& 2.25 	& 0.082	& 0.075 \\
%RandomForest   & 0.51    & 1.75 & 0.127   & 0.127   & 0.62    & 1.33 & 0.092   & 0.092    \\ 
%SVM            & 0.72    & 1.34 & 0.097   & 0.097   & 0.73    & 1.18 & 0.080   & 0.080    \\ 
%XGBoost        & 0.46    & 1.63 & 0.118   & 0.118   & 0.64    & 1.25 & 0.086   & 0.086    \\ 
%DeepAR         & 0.66    & 2.07 & 0.156   & 0.096   & 0.59    & 1.71 & 0.121   & 0.075    \\ 
%RankNet-Joint  & 0.73    & 1.75 & 0.140   & 0.086   & 0.68    & 1.63 & 0.116   & 0.073    \\  \hline
%RankNet-MLP    &\textbf{0.77}    & \textbf{1.24} & \textbf{0.086}   & \textbf{0.077}   & \textbf{0.78}    & \textbf{1.07} & \textbf{0.072}   & \textbf{0.061}    \\
%\hline
%RankNet-Oracle & 0.85    & 1.11 & 0.080   & 0.073   & 0.86    & 0.98 & 0.067   & 0.061    \\

%\hline
%\end{tabular}
%\end{table*}

\begin{table}[ht]

\centering
\caption{Short-term rank position forecasting(prediction leghth=2) Indy500-2019}
\label{tbl:rank_forecasting}
\begin{tabular}{l|llll} 

\hline
Model            & Top1Acc & MAE  & 50-Risk & 90-Risk         \\ 
\hline
CurRank          & 0.73    & 1.16 & 0.080   & 0.080    \\ 
ARIMA		& 0.57	& 2.25 	& 0.082	& 0.075 \\
RandomForest     & 0.62    & 1.33 & 0.092   & 0.092    \\ 
SVM               & 0.73    & 1.18 & 0.080   & 0.080    \\ 
XGBoost          & 0.64    & 1.25 & 0.086   & 0.086    \\ 
DeepAR            & 0.59    & 1.71 & 0.121   & 0.075    \\ 
RankNet-Joint    & 0.68    & 1.63 & 0.116   & 0.073    \\  \hline
RankNet-MLP     & \textbf{0.78}    & \textbf{1.07} & \textbf{0.072}   & \textbf{0.061}    \\
\hline
RankNet-Oracle   & 0.86    & 0.98 & 0.067   & 0.061    \\

\hline
\end{tabular}
\end{table}
\fi

\begin{table*}
\small
\centering
\caption{Short-term rank position forecasting(prediction leghth=2) of Indy500-2019}

\begin{tabular}{l|llll|llll} 
\hline
Dataset   & \multicolumn{4}{c|}{Normal lap} & \multicolumn{4}{c}{Lap with events}  \\ 
\hline
Model   & SignAcc & MAE  & 50-Risk & 90-Risk    & SignAcc & MAE  & 50-Risk & 90-Risk \\ 
\hline
CurRank &0.95   &0.11   &0.01    &0.01    &0.60    &1.86    &0.13    &0.13\\
RandomForest    & 0.80  &0.38   &0.03  &0.03 &0.51    &1.93   &0.13  &0.13\\
SVM &   0.95  &0.11 &0.01    &0.01   &0.59  &1.86 &0.13    &0.13\\
XGBoost & 0.79&0.23 &0.02   &0.02   &0.55   &1.92   &0.13   &0.13\\
\hline

RankNet-MLP & 0.93  &0.17   &0.01   &0.01   &\textbf{0.67}  &\textbf{1.67}   &\textbf{0.11}   &\textbf{0.09}\\
\hline
RankNet-Oracle  & 0.93  &0.17   &0.01  &0.01 &0.81   &1.50  &0.10 &0.09\\
\hline
\end{tabular}
\end{table*}

begin{table}

\centering
\caption{Rank position changes forecasting between pit stops}
\label{tbl:rank_change}
\begin{tabular}{l|llll} 

\hline
Model          & SignAcc & MAE  & 50-Risk & 90-Risk     \\ 
\hline
CurRank   & 0.15 & 4.33                     & 0.280                        & 0.262                         \\ 
RandomForest & 0.51                         & 4.31                     & 0.277                        & 0.276                         \\ 
SVM & 0.51                         & 4.22                     & 0.270 & 0.249 \\ 
XGBoost & 0.45 & 4.86 & 0.313 & 0.304 \\ 
\hline
 
RankNet-MLP     & \textbf{0.62}  & \textbf{4.33} & \textbf{0.286} & \textbf{0.223} \\
\hline
RankNet-Oracle & 0.66                         & 3.62                     & 0.234                        & 0.215                         \\ 
\hline
\end{tabular}
\end{table}

\begin{figure*}[hbt]
\centering
\label{fig:modelopt}
\includegraphics[width=1\linewidth]{fig/modeloptimize_onerow.pdf}
\caption{Illustration of RankNet model optimization on two laps forecasting for Car13 Indy500-2018.(a)Basic RankNet model trained with Oracle race status features and context\_length=40. (b)Adding larger weights to the loss for instances with rank changes. (c)Tuning on parameter context\_length, set optimal length to 60. (d)Adding context features, including leader\_pit\_cnt: \# of leading cars(based on the rank position at lap A-2) that go to pit stop at lap A; total\_pit\_cnt:\# of cars that go to pit stop at lap A. (e)Adding shift features, including shift\_racestatus: lapstatus and trackstatus of the future at lap A+2;
shift\_total\_pit\_cnt:\# of cars that go to pit stop at lap A+2.}
\end{figure*}

\begin{table*}
\centering
\caption{IndyCar Dataset}
\label{tbl:dataset}
\begin{tabular}{lllllllllll} 
\hline
Race & Year& Track Length &Track Shape & Total Laps & Avg Speed &\# Participants   & \# Records &Training & Validation&Test \\
\hline
Indy500& 2013-2019 & 2.5& Oval &200 & 175mph &33    & 6600 & \checkmark & &  \\ 
%Indy500& 2018 & 2.5& Oval &200 & 175mph &33   & 6600 &  & \checkmark &  \\ 
%Indy500& 2019 & 2.5& Oval &200 & 175mph &33   & 6600 &  & &  \checkmark \\ 
%Gateway&2018 & 1.25& Oval &248  & 185mph & 21  &5208 &&&  \checkmark\\ 
%Gateway&2019 & 1.25& Oval &248  & 185mph & 22  &5456 &&&  \checkmark\\ 
Iowa&  2013  & 0.894& Oval&250&135mph& 24  & 6000&&& \checkmark\\ 
Iowa&  2015-2019  & 0.894& Oval&300&135mph& 21-24  & 7200&&& \checkmark\\ 
%Phoenix& 2018& 1.02& Oval &250 &105mph & 23  &5750&&& \checkmark\\ 
Pocono&2013  & 2.5 & Triangle &160 & 135mph & 24   &3840&&& \checkmark\\ 
Pocono&2015-2018  & 2.5& Triangle  &200 & 135mph & 22-24   &4800&&& \checkmark\\ %Pocono&2019  & 2.5  &128 & 135mph & 22   &2816&&& \checkmark\\ 
Texas & 2013 & 1.455& Oval &228 & 153mph & 24   & 5472&&& \checkmark\\
Texas & 2014-2019 & 1.455 & Oval&248 & 153mph & 22-23   & 5704&&& \checkmark\\
\hline
\end{tabular}
\end{table*}
